# Supplementary material for: Explaining the Ubiquity of Phase Transitions in Decision Problems
Source: arXiv:2501.14569 source file (2025-01-24)
Supplement: Supplementary file 1 [file TogoodForm.tex]

\label{ToGoodForm}
\begin{theorem}
    Given an parameter, $\tau$, such that the acceptence fraction, $\mathcal{A}$, obeys the following:
    \begin{align}
            &\bullet \mathcal{A} > 1 - c^{\tau^2} \textit{  if } \tau > 0\\
            &\bullet \mathcal{A} < c^{\tau^2} \textit{  if } \tau > 1\\
            &\bullet \lim_{\tau \rightarrow 0^+} \big( \mathcal{A} \big) = 0\\
            &\bullet \lim_{\tau \rightarrow 0^-} \big( \mathcal{A} \big) = 1
    \end{align}
    Then it is possible to construct an parameter, $\tau^{\prime}$, such that:
\end{theorem}
\begin{lemma}
    \label{properFormLemma}
\end{lemma}
\begin{proof}
    Solve $\frac{7}{2}c^n = \frac{1}{2}$, for $c$, and define $k = \dfrac{1}{\sqrt{2}} \geq c$, therefore:
    \begin{align}
        c^n &= \frac{1}{7}
        \Rightarrow
        K^n \geq \frac{1}{7}
        \Rightarrow
        n = \log_{K} \bigg( \frac{1}{7} \bigg)
        \approx 5.6147
    \end{align}
    We use this calculation to ``pull-in" the bounds of the transition by defining:
    \begin{align}
       \vert \tau^{\dagger} \vert
       &=
       \vert \tau \vert - 6
    \end{align}
    if $\vert \tau \vert \geq 6$. For the inputs with  $\vert \tau \vert < 6$, we use a different process. As there are finitely many such inputs, we can simply assign their positions to reinforce the bounds via a list of what $\tau$ values to assign them, knowing their correct outputs.\\
    The only requirement on this is that we must ensure that exactly half of the inputs mapped to $\tau = 0$ are in the language and half are not in the language.
\end{proof}
